# Supplementary material for: ZiGAN: Fine-grained Chinese Calligraphy Font Generation via a Few-shot Style Transfer Approach
Source: arXiv:2108.03596 source file (2021-08-08)
Supplement: Supplementary file 1 [file 06-Supplementary.tex]

% \clearpage
\section*{Supplementary}

\noindent\textbf{Fréchet Inception Distance} For quantitative evaluation, we also use Fréchet Inception Distance to measure whether our results have completed the style translation. FID calculates the distance between the real image and the generated image in the feature space. And the feature representations are extracted from the Inception network. The lower the value indicates that the distribution of the generated images is closer to the real images distribution, and the result is better. As above, we compare six classic methods, and Table \ref{tab:FID} shows that ZiGAN achieves the lowest FID scores.

\noindent\textbf{Additional Experimental Results} In addition to the results presented in the paper, we randomly select 50 common characters for each font with different styles and show supplement generation results for the datasets in Figure \ref{fig:result1} and Figure \ref{fig:result2}.
\\

\begin{table*}[]
    \centering
    \setlength{\tabcolsep}{2.3mm}{

    \caption{Fréchet Inception Distance for difference font style translation mode. Lower is better. The seventh and eighth methods show the results of ablation experiments without $\mathcal{L}_{style}$ or $\mathcal{L}_{alignment}$.}
    \label{tab:FID}
    \small
    \begin{tabular}{m{6mm}|c|m{12mm}<{\centering}|m{12mm}<{\centering}|m{12mm}<{\centering}|m{12mm}<{\centering}|m{12mm}<{\centering}|m{12mm}<{\centering}|m{12mm}<{\centering}|m{12mm}<{\centering}}
        \hline
        \multicolumn{10}{c}{\textbf{Fréchet Inception Distance ~ (FID)}} \\
        \hline
        \multirow{2}{*}{Type} & \multirow{2}{*}{Method}
        & \multicolumn{8}{c}{Style} \\
        \cline{3-10}
        & & 1 & 2 & 3 & 4 & 5 & 6 & 7 & Mean \\
        \hline
        \multirow{9}{*}{\tabincell{c}{100 \\ - \\ shot}}
        & zi2zi & 2.164 & 2.589 & 2.348 & 2.385 & 2.494 & 2.359 & 2.196 & 2.362  \\
        & pix2pix & 1.789 & 1.739 & 2.335 & 2.322 & 2.208 & 1.574 & 2.318 & 2.041 \\
        & U-GAT-IT & 1.222 & 0.904 & 1.273 & 0.920 & \textbf{0.968} & 1.218 & 1.288 & 1.113 \\
        & CycleGAN & 1.608 & 2.743 & 1.480 & 1.659 & 2.425 & 1.230 & 1.707 & 1.836 \\
        & StarGAN & 2.053 & 2.899 & 2.396 & 2.385 & 2.731 & 2.295 & 2.590 & 2.478 \\
        & CalliGAN & 2.091 & 2.527 & 2.340 & 2.355 & 2.366 & 2.201 & 2.142 & 2.289\\
        & ZiGAN w/o $\mathcal{L}_{style}$ & 1.254 & 1.842 & 1.827 & 1.779 & 2.759 & 1.914 & 1.6 & 1.854 \\
        & ZiGAN w/o $\mathcal{L}_{align}$ & 1.312 & 1.924 & 1.586 & 1.547 & 1.874 & 1.368 & 1.252 & 1.552 \\
        & \textbf{ZiGAN(Ours)} & \textbf{1.047} & \textbf{0.845} & \textbf{0.816} & \textbf{0.816} & 1.189 & \textbf{1.109} & \textbf{0.669} & \textbf{0.927} \\
        \hline
        \multirow{9}{*}{\tabincell{c}{200 \\ - \\ shot}}
        & zi2zi & 1.380 & 0.756 & 1.649 & 1.010 & 1.270 & 1.119 & 1.359 & 1.220 \\
        & pix2pix & 0.966 & 1.024 & 1.021 & 1.290 & 0.985 & 0.831 & 1.138 & 1.036 \\
        & U-GAT-IT & 1.065 & 0.691 & 0.583 & 0.662 & \textbf{0.667} & 0.689 & 0.686 & 0.720 \\
        & CycleGAN & 1.293 & 2.268 & 1.028 & 2.159 & 2.189 & 1.380 & 1.420 & 1.677 \\
        & StarGAN & 2.456 & 2.757 & 2.373 & 2.497 & 2.370 & 2.180 & 2.342 & 2.425 \\
        & CalliGAN & 1.331 & 1.808 & 1.615 & 0.916 & 1.423 & 1.001 & 1.208 & 1.329 \\
        & ZiGAN w/o $\mathcal{L}_{style}$ & 1.019 & 0.889 & 0.973 & 0.991 & 1.302 & 0.817 & 0.879 & 0.987 \\
        & ZiGAN w/o $\mathcal{L}_{align}$ & 0.517 & \textbf{0.582} & 0.616 & \textbf{0.574} & 0.883 & 0.720 & 0.729 & 0.660 \\
        & \textbf{ZiGAN(Ours)} & \textbf{0.279} & 0.868 & \textbf{0.476} & 0.678 & 0.687 & \textbf{0.663} & \textbf{0.654} & \textbf{0.615} \\
        \hline
    \end{tabular}}
\end{table*}

\begin{figure*}[ht]
    \centering
    \begin{tabular}{c}
        \toprule
        \vspace{-0.5em}
        \includegraphics[height=2cm]{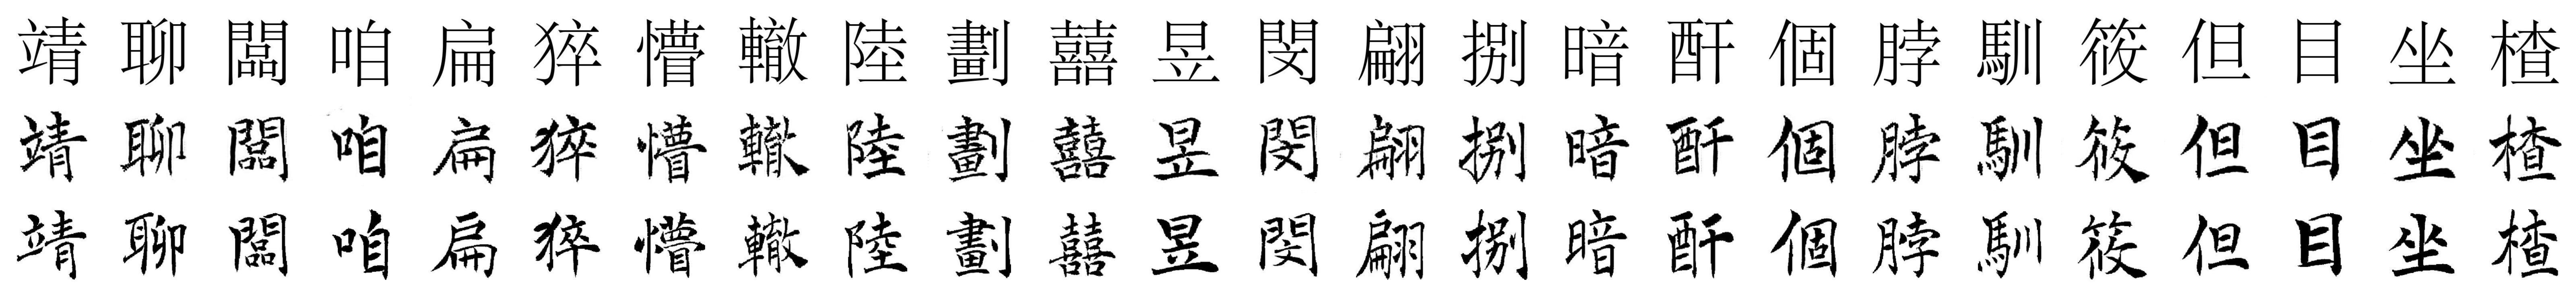} \\
        \includegraphics[height=2cm]{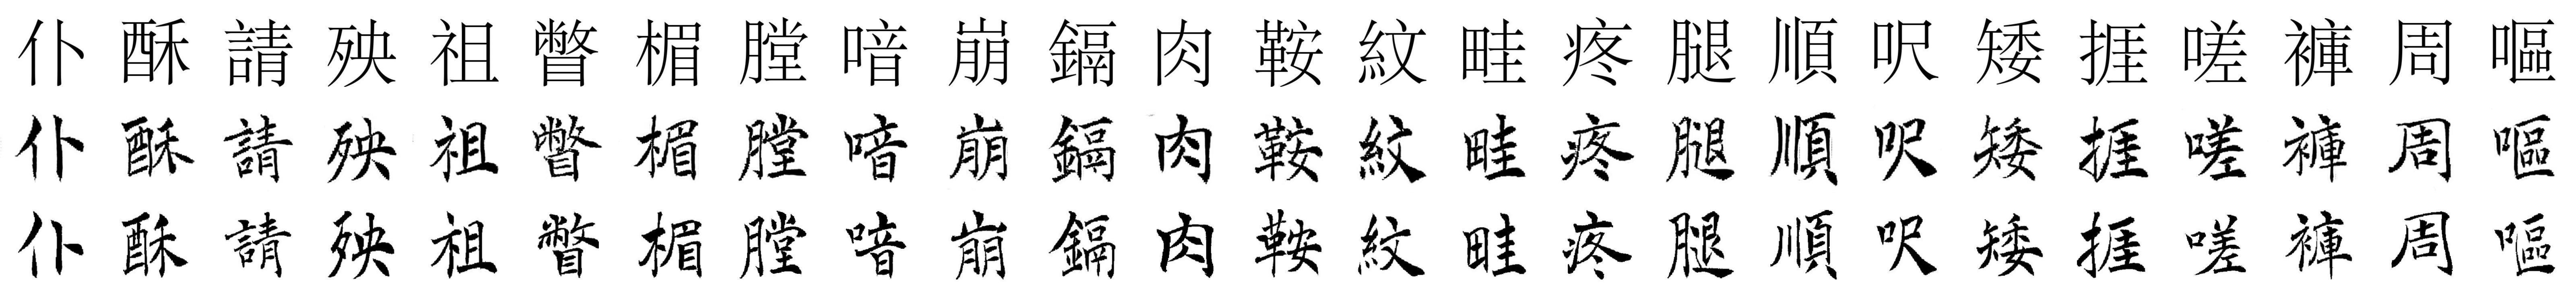} \\
        \toprule
        \vspace{-0.5em}
        \includegraphics[height=2cm]{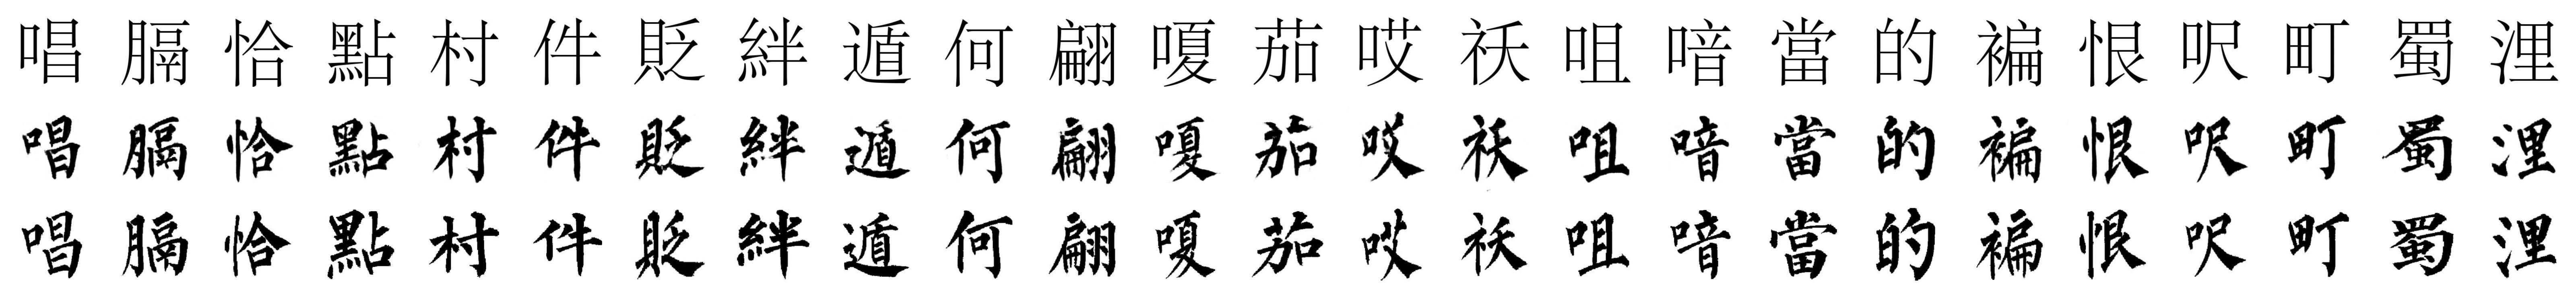} \\
        \includegraphics[height=2cm]{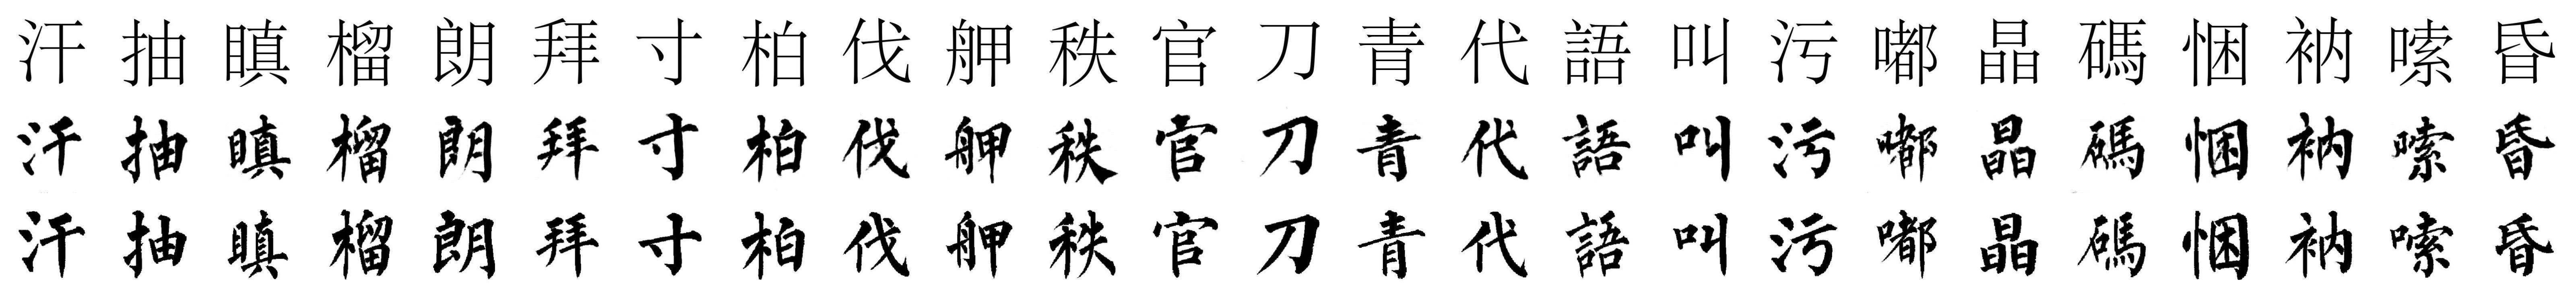} \\
        \toprule
        \vspace{-0.5em}
        \includegraphics[height=2cm]{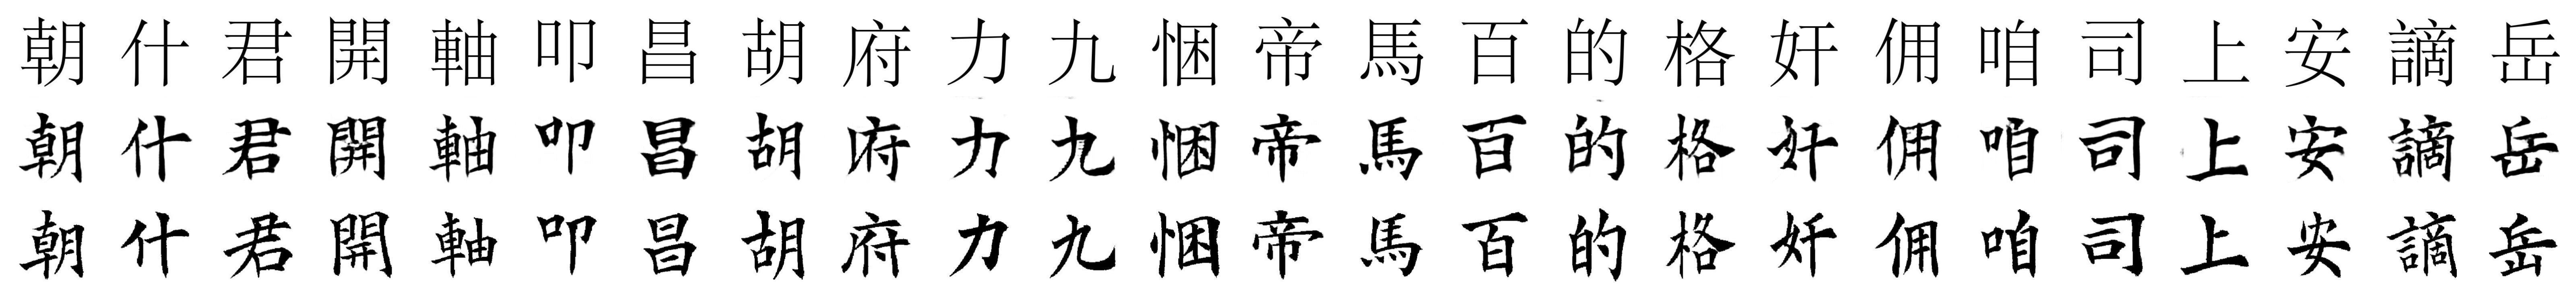} \\
        \includegraphics[height=2cm]{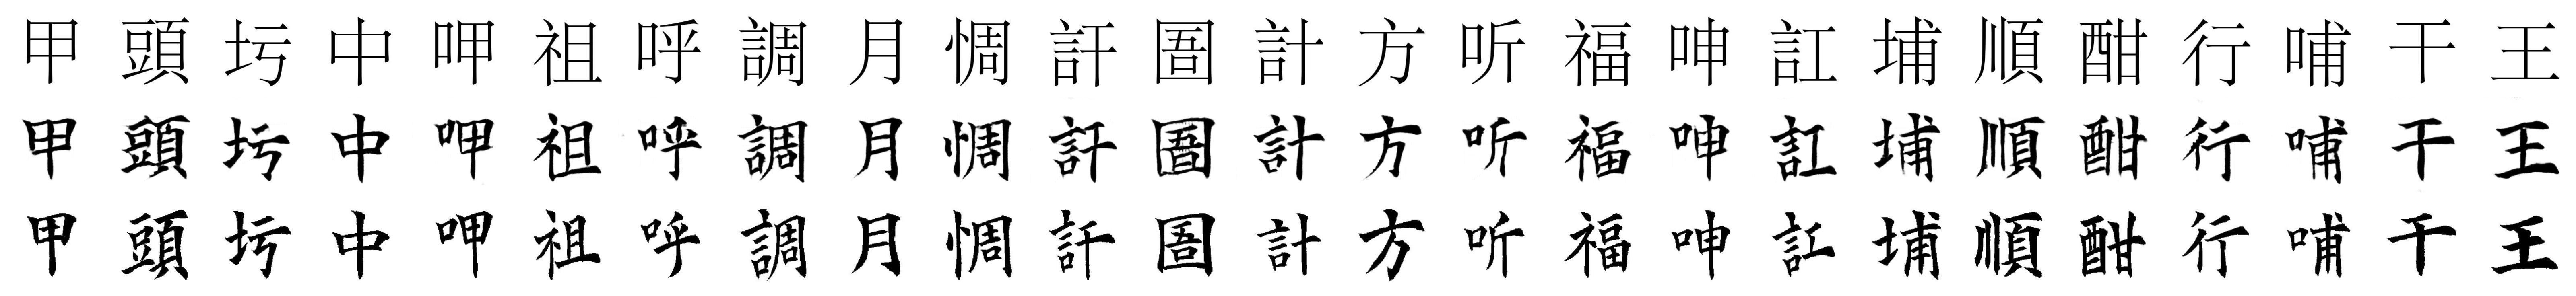} \\
        \toprule
        \vspace{-0.5em}
        \includegraphics[height=2cm]{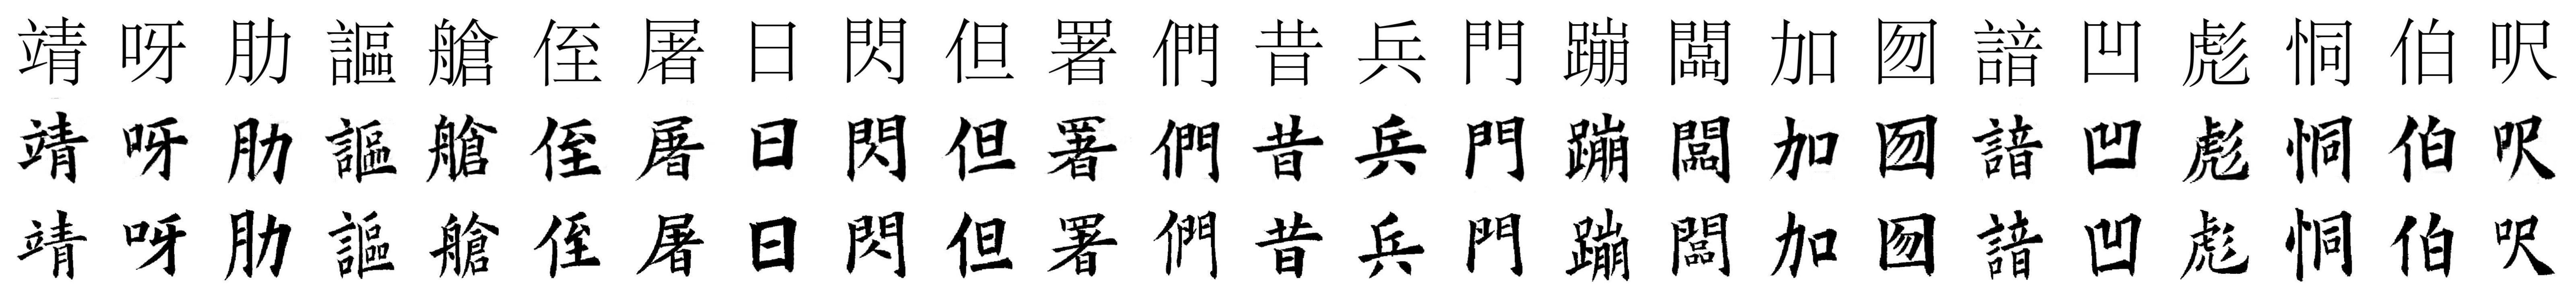} \\
        \includegraphics[height=2cm]{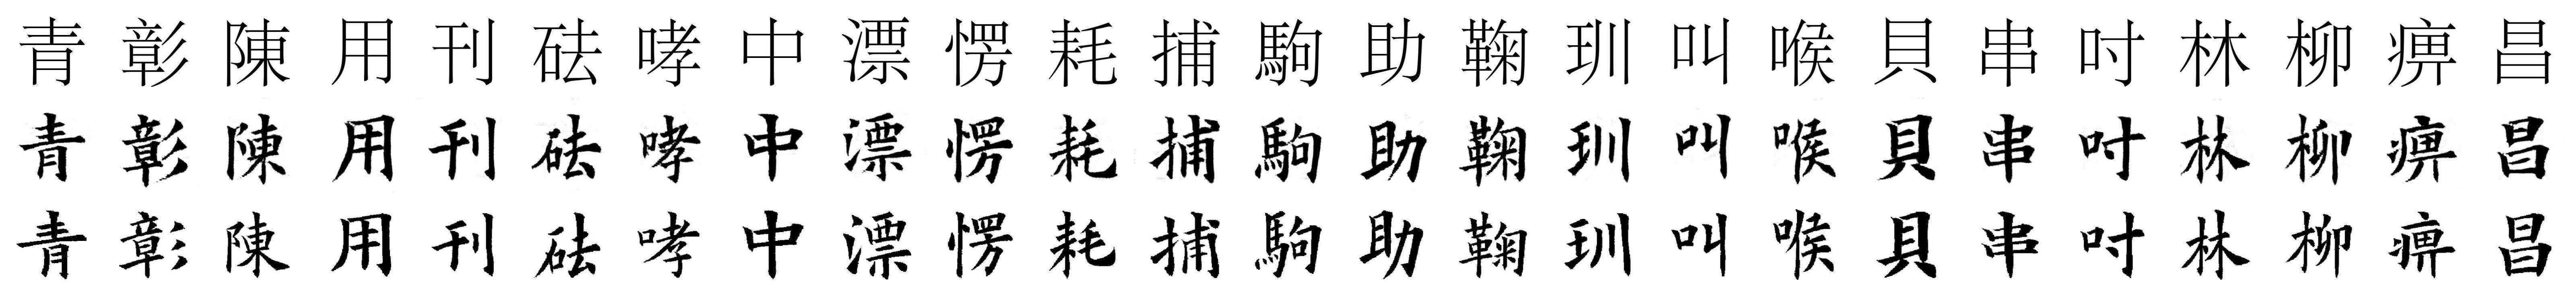} \\
        \toprule
        \vspace{-0.5em}
        \includegraphics[height=2cm]{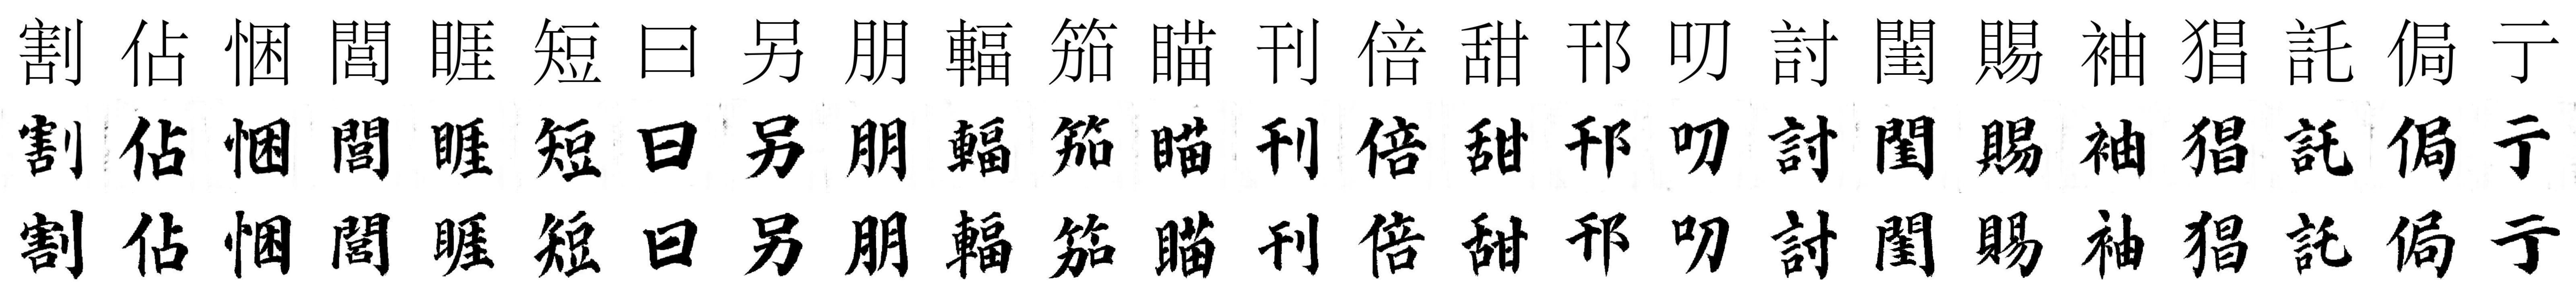} \\
        \includegraphics[height=2cm]{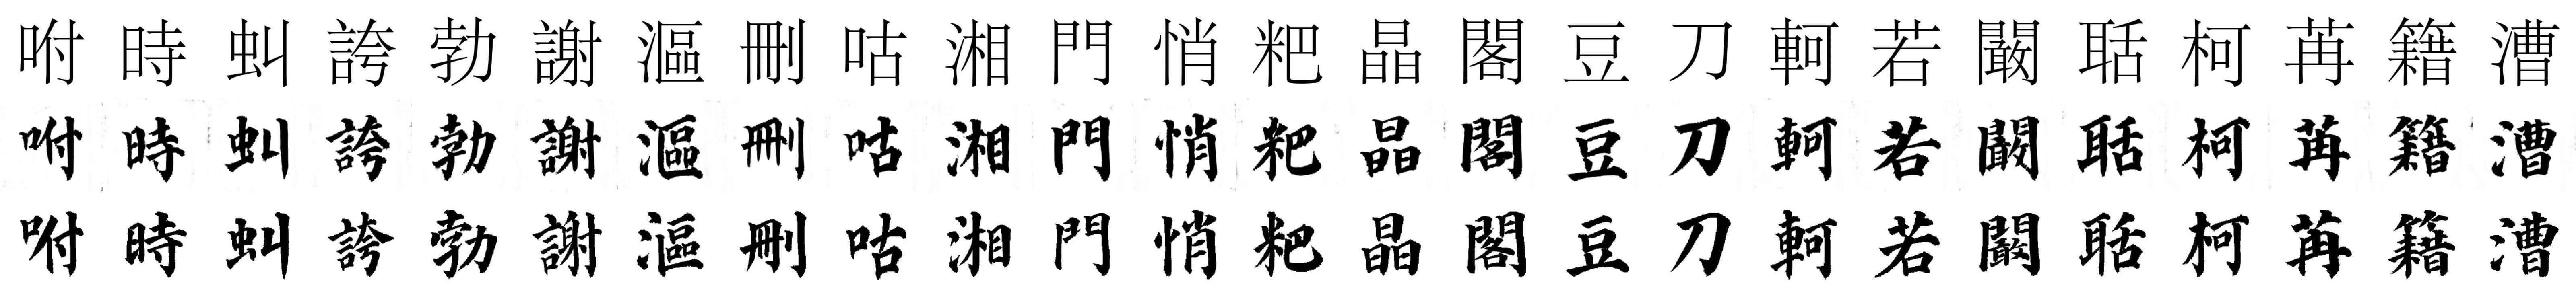} \\
        \toprule
    \end{tabular}
    \caption{ Visual comparison of the results of the first to fifth styles. The first row shows the source characters. The second row shows the characters generated by ZiGAN. And the third row shows the ground truth.}
    \label{fig:result1}
    % \vspace{-1em}
\end{figure*}

\begin{figure*}[ht]
    \centering
    \begin{tabular}{c}
        \toprule
        \vspace{-0.5em}
        \includegraphics[height=2cm]{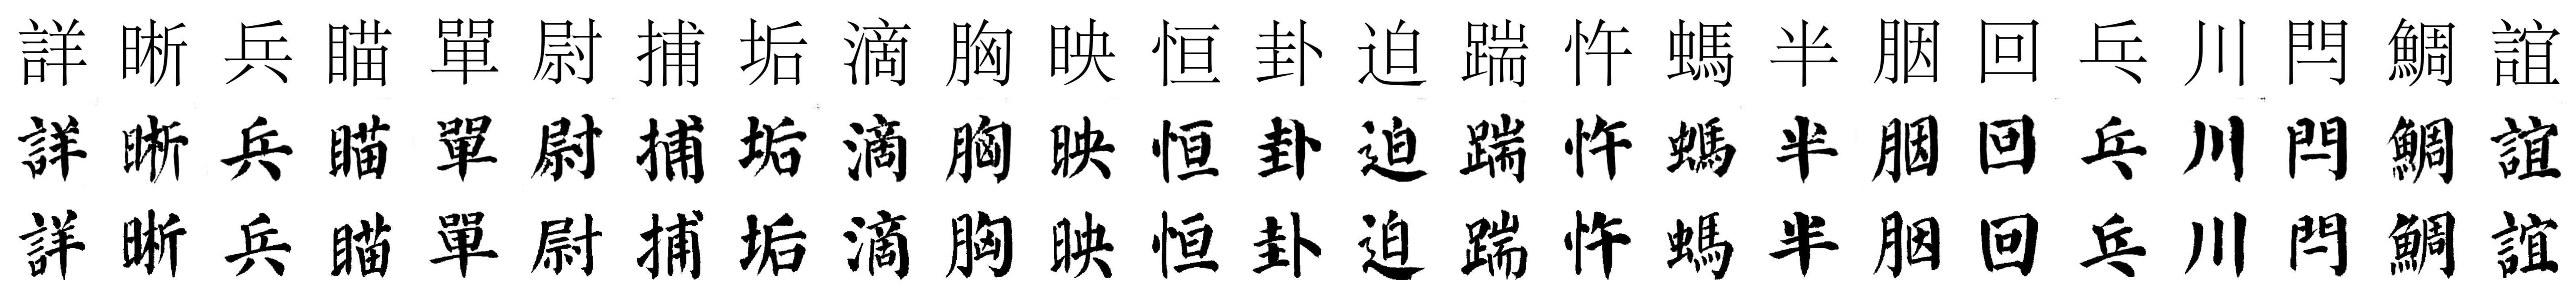} \\
        \includegraphics[height=2cm]{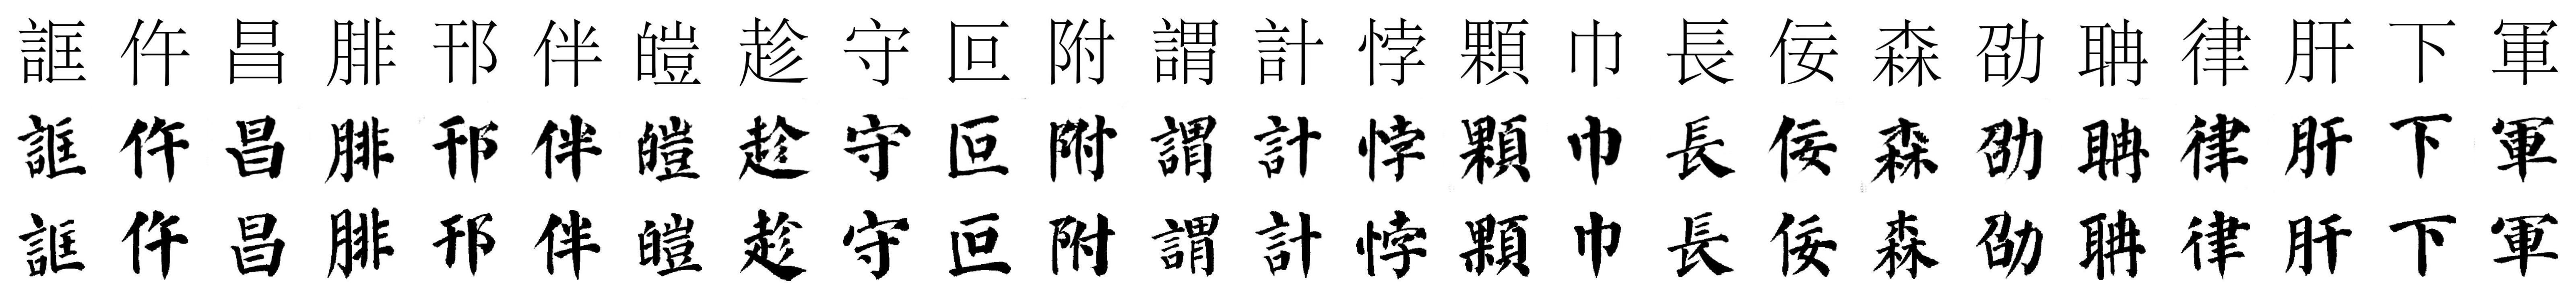} \\
        \toprule
        \vspace{-0.5em}
        \includegraphics[height=2cm]{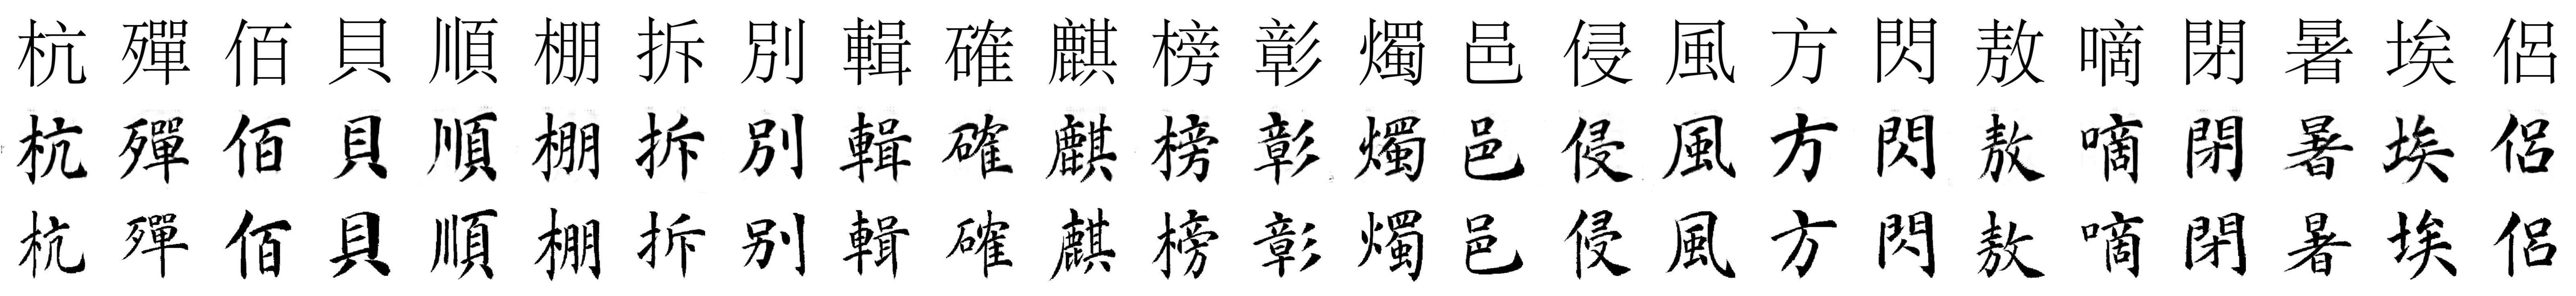} \\
        \includegraphics[height=2cm]{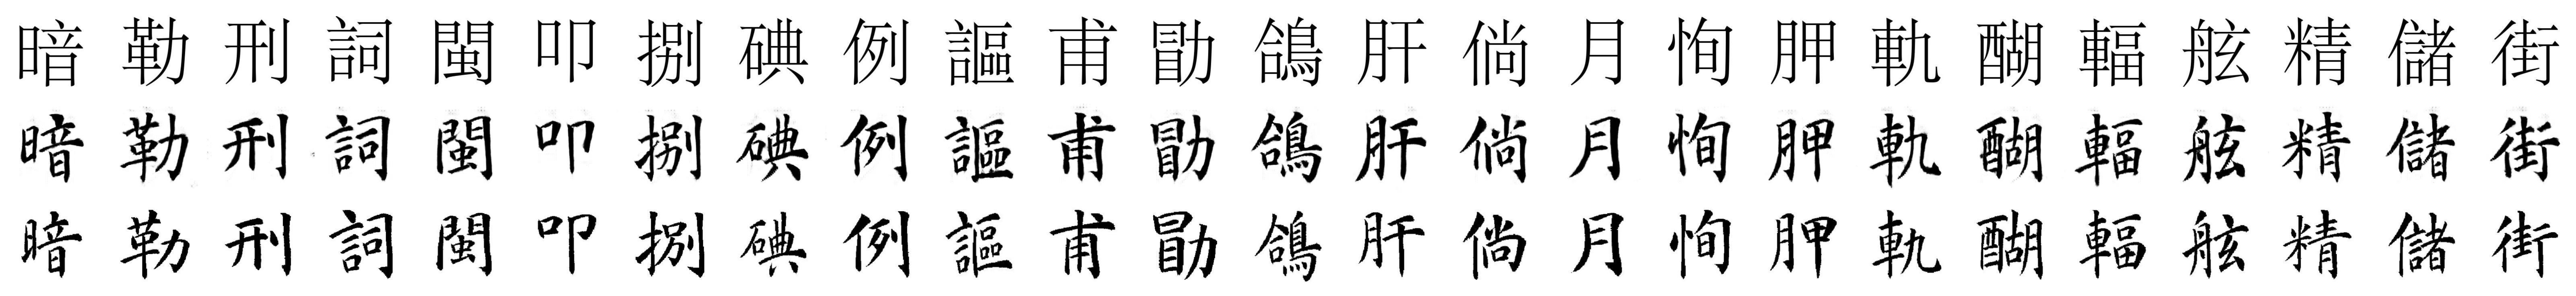} \\
        \toprule
        \vspace{-0.5em}
        \includegraphics[height=2cm]{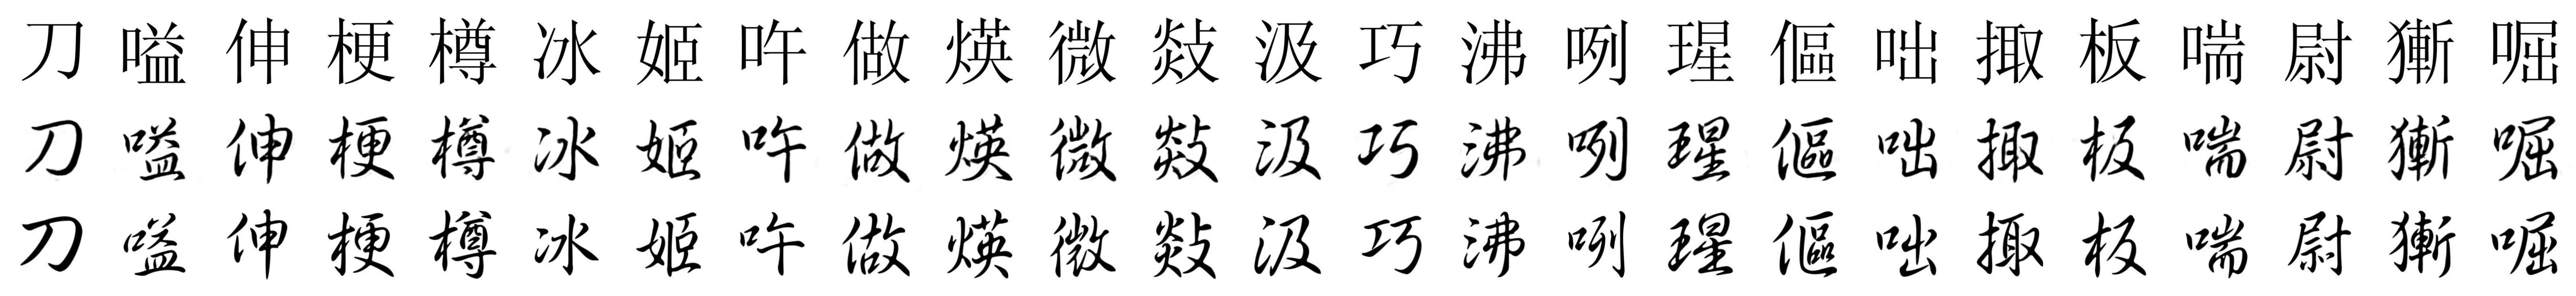} \\
        \includegraphics[height=2cm]{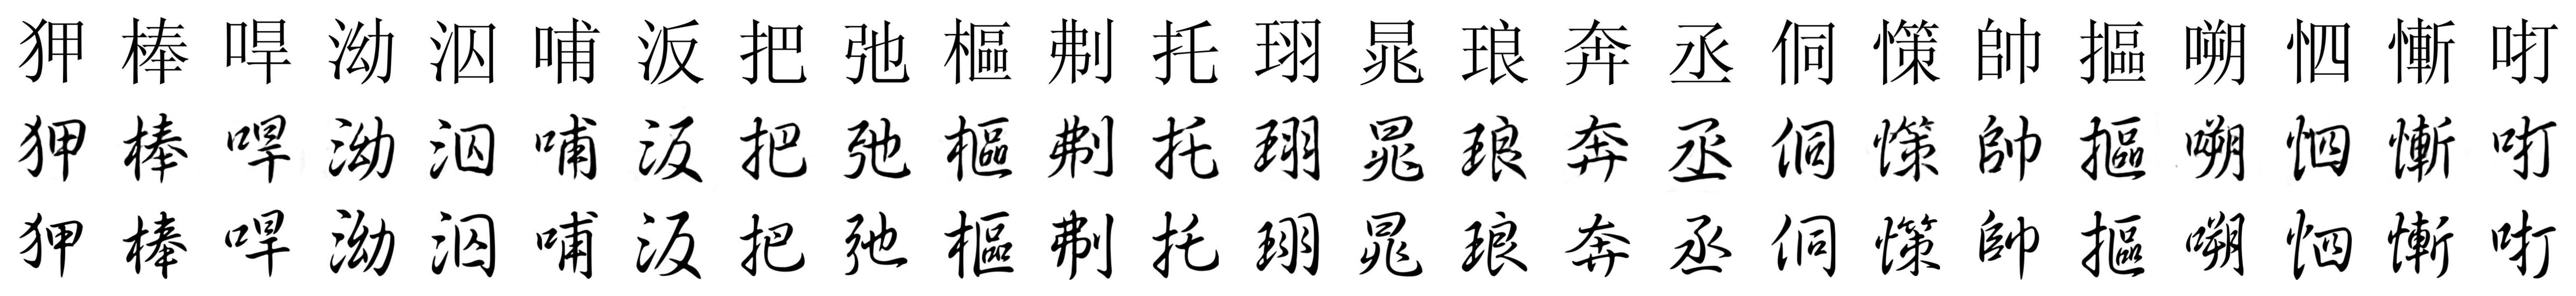} \\
        \toprule
        \vspace{-0.5em}
        \includegraphics[height=2cm]{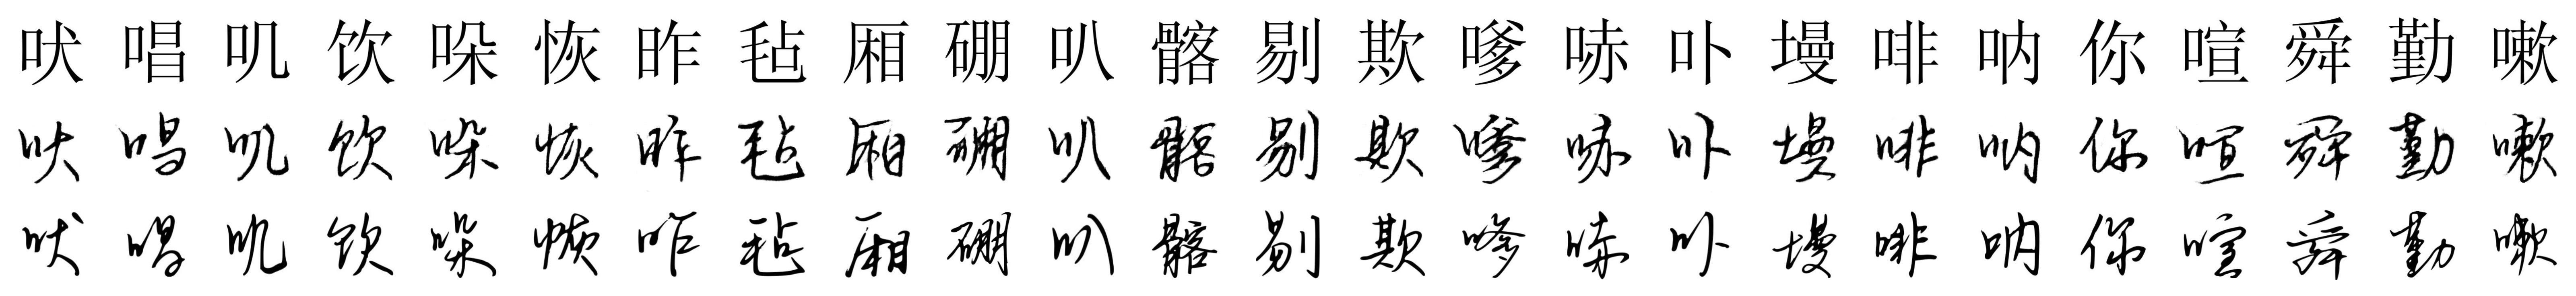} \\
        \includegraphics[height=2cm]{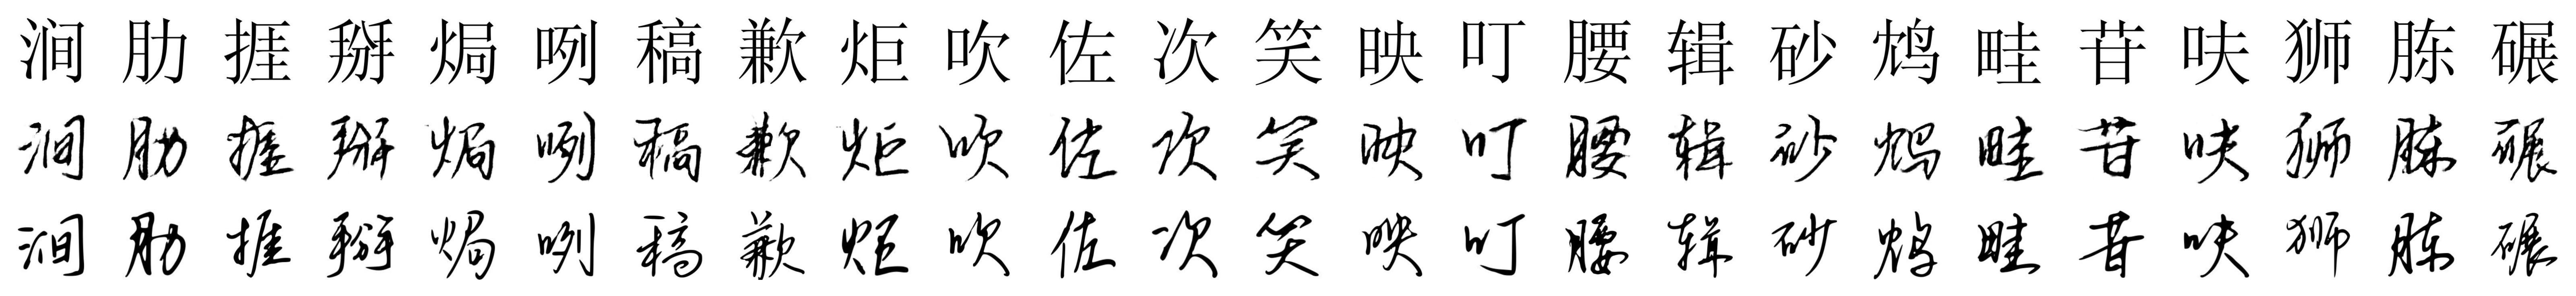} \\
        \toprule
    \end{tabular}
    \caption{ Visual comparison of the results of the sixth to ninth styles. The first row shows the source characters. The second row shows the characters generated by ZiGAN. And the third row shows the ground truth.}
    \label{fig:result2}
    % \vspace{-1em}
\end{figure*}
