# Supplementary material for: ZiGAN: Fine-grained Chinese Calligraphy Font Generation via a Few-shot Style Transfer Approach
Source: arXiv:2108.03596 source file (2021-08-08)
Supplement: Supplementary file 2 [file ZiGAN_SUPPLEMENTARY.pdf]

# ZiGAN: Fine-grained Chinese Calligraphy Font Generation via a Few-shot Style Transfer Approach

Qi Wen\*  
wenqijay@gmail.com  
NetEase Fuxi AI Lab  
Hangzhou, China

Bingfeng Han  
bfhan@bit.edu.cn  
Beijing Institute of Technology  
Beijing, China

Shuang Li\*  
shuangli@bit.edu.cn  
Beijing Institute of Technology  
Beijing, China

Yi Yuan†  
yuanyi@corp.netease.com  
NetEase Fuxi AI Lab  
Hangzhou, China

## ACM Reference Format:

Qi Wen, Shuang Li, Bingfeng Han, and Yi Yuan. 2021. ZiGAN: Fine-grained Chinese Calligraphy Font Generation via a Few-shot Style Transfer Approach. In *Proceedings of the 29th ACM Int'l Conference on Multimedia (MM '21), Oct. 20–24, 2021, Virtual Event, China*. ACM, New York, NY, USA, 4 pages. <https://doi.org/10.1145/3474085.3475225>

## SUPPLEMENTARY

**Fréchet Inception Distance** For quantitative evaluation, we also use Fréchet Inception Distance to measure whether our results have completed the style translation. FID calculates the distance between the real image and the generated image in the feature space. And the feature representations are extracted from the Inception network. The lower the value indicates that the distribution of the generated images is closer to the real images distribution, and the result is better. As above, we compare six classic methods, and Table 1 shows that ZiGAN achieves the lowest FID scores.

**Additional Experimental Results** In addition to the results presented in the paper, we randomly select 50 common characters for each font with different styles and show supplement generation results for the datasets in Figure 1 and Figure 2.

---

\*Authors contribute equally.

†Dr. Yuan is the corresponding author.

---

Permission to make digital or hard copies of all or part of this work for personal or classroom use is granted without fee provided that copies are not made or distributed for profit or commercial advantage and that copies bear this notice and the full citation on the first page. Copyrights for components of this work owned by others than ACM must be honored. Abstracting with credit is permitted. To copy otherwise, or republish, to post on servers or to redistribute to lists, requires prior specific permission and/or a fee. Request permissions from [permissions@acm.org](mailto:permissions@acm.org).

MM '21, October 20–24, 2021, Virtual Event, China.

© 2021 Association for Computing Machinery.

ACM ISBN 978-1-4503-8651-7/21/10...\$15.00

<https://doi.org/10.1145/3474085.3475225>

**Table 1: Fréchet Inception Distance for difference font style translation mode. Lower is better. The seventh and eighth methods show the results of ablation experiments without  $\mathcal{L}_{style}$  or  $\mathcal{L}_{alignment}$ .**

| Fréchet Inception Distance (FID) |                                 |              |              |              |              |              |              |              |              |
|----------------------------------|---------------------------------|--------------|--------------|--------------|--------------|--------------|--------------|--------------|--------------|
| Type                             | Method                          | Style        |              |              |              |              |              |              | Mean         |
|                                  |                                 | 1            | 2            | 3            | 4            | 5            | 6            | 7            |              |
| 100<br>-<br>shot                 | zi2zi                           | 2.164        | 2.589        | 2.348        | 2.385        | 2.494        | 2.359        | 2.196        | 2.362        |
|                                  | pix2pix                         | 1.789        | 1.739        | 2.335        | 2.322        | 2.208        | 1.574        | 2.318        | 2.041        |
|                                  | U-GAT-IT                        | 1.222        | 0.904        | 1.273        | 0.920        | <b>0.968</b> | 1.218        | 1.288        | 1.113        |
|                                  | CycleGAN                        | 1.608        | 2.743        | 1.480        | 1.659        | 2.425        | 1.230        | 1.707        | 1.836        |
|                                  | StarGAN                         | 2.053        | 2.899        | 2.396        | 2.385        | 2.731        | 2.295        | 2.590        | 2.478        |
|                                  | CalliGAN                        | 2.091        | 2.527        | 2.340        | 2.355        | 2.366        | 2.201        | 2.142        | 2.289        |
|                                  | ZiGAN w/o $\mathcal{L}_{style}$ | 1.254        | 1.842        | 1.827        | 1.779        | 2.759        | 1.914        | 1.6          | 1.854        |
|                                  | ZiGAN w/o $\mathcal{L}_{align}$ | 1.312        | 1.924        | 1.586        | 1.547        | 1.874        | 1.368        | 1.252        | 1.552        |
|                                  | <b>ZiGAN(Ours)</b>              | <b>1.047</b> | <b>0.845</b> | <b>0.816</b> | <b>0.816</b> | 1.189        | <b>1.109</b> | <b>0.669</b> | <b>0.927</b> |
| 200<br>-<br>shot                 | zi2zi                           | 1.380        | 0.756        | 1.649        | 1.010        | 1.270        | 1.119        | 1.359        | 1.220        |
|                                  | pix2pix                         | 0.966        | 1.024        | 1.021        | 1.290        | 0.985        | 0.831        | 1.138        | 1.036        |
|                                  | U-GAT-IT                        | 1.065        | 0.691        | 0.583        | 0.662        | <b>0.667</b> | 0.689        | 0.686        | 0.720        |
|                                  | CycleGAN                        | 1.293        | 2.268        | 1.028        | 2.159        | 2.189        | 1.380        | 1.420        | 1.677        |
|                                  | StarGAN                         | 2.456        | 2.757        | 2.373        | 2.497        | 2.370        | 2.180        | 2.342        | 2.425        |
|                                  | CalliGAN                        | 1.331        | 1.808        | 1.615        | 0.916        | 1.423        | 1.001        | 1.208        | 1.329        |
|                                  | ZiGAN w/o $\mathcal{L}_{style}$ | 1.019        | 0.889        | 0.973        | 0.991        | 1.302        | 0.817        | 0.879        | 0.987        |
|                                  | ZiGAN w/o $\mathcal{L}_{align}$ | 0.517        | <b>0.582</b> | 0.616        | <b>0.574</b> | 0.883        | 0.720        | 0.729        | 0.660        |
|                                  | <b>ZiGAN(Ours)</b>              | <b>0.279</b> | 0.868        | <b>0.476</b> | 0.678        | 0.687        | <b>0.663</b> | <b>0.654</b> | <b>0.615</b> |

|   |   |   |   |   |   |   |   |   |   |   |   |   |   |   |   |   |   |   |   |   |   |   |   |   |
|---|---|---|---|---|---|---|---|---|---|---|---|---|---|---|---|---|---|---|---|---|---|---|---|---|
| 靖 | 聊 | 闊 | 咱 | 扁 | 猝 | 懣 | 轍 | 陸 | 劃 | 囍 | 昱 | 閔 | 翩 | 捌 | 暗 | 酩 | 個 | 脖 | 馴 | 筱 | 但 | 目 | 坐 | 楂 |
| 靖 | 聊 | 闊 | 咱 | 扁 | 猝 | 懣 | 轍 | 陸 | 劃 | 囍 | 昱 | 閔 | 翩 | 捌 | 暗 | 酩 | 個 | 脖 | 馴 | 筱 | 但 | 目 | 坐 | 楂 |
| 靖 | 聊 | 闊 | 咱 | 扁 | 猝 | 懣 | 轍 | 陸 | 劃 | 囍 | 昱 | 閔 | 翩 | 捌 | 暗 | 酩 | 個 | 脖 | 馴 | 筱 | 但 | 目 | 坐 | 楂 |
| 仆 | 酥 | 請 | 殃 | 祖 | 瞥 | 楣 | 膛 | 暗 | 崩 | 鐳 | 肉 | 鞍 | 紋 | 畦 | 疼 | 腿 | 順 | 呎 | 矮 | 握 | 嗟 | 褲 | 周 | 嘔 |
| 仆 | 酥 | 請 | 殃 | 祖 | 瞥 | 楣 | 膛 | 暗 | 崩 | 鐳 | 肉 | 鞍 | 紋 | 畦 | 疼 | 腿 | 順 | 呎 | 矮 | 握 | 嗟 | 褲 | 周 | 嘔 |
| 唱 | 膈 | 恰 | 點 | 村 | 件 | 貶 | 絆 | 遁 | 何 | 翩 | 噯 | 茄 | 哎 | 袄 | 咀 | 暗 | 當 | 的 | 編 | 恨 | 呎 | 町 | 蜀 | 涇 |
| 唱 | 膈 | 恰 | 點 | 村 | 件 | 貶 | 絆 | 遁 | 何 | 翩 | 噯 | 茄 | 哎 | 袄 | 咀 | 暗 | 當 | 的 | 編 | 恨 | 呎 | 町 | 蜀 | 涇 |
| 汗 | 抽 | 瞋 | 榴 | 朗 | 拜 | 寸 | 柏 | 伐 | 舛 | 秩 | 官 | 刀 | 青 | 代 | 語 | 叫 | 污 | 的 | 晶 | 碼 | 惆 | 衲 | 唻 | 昏 |
| 汗 | 抽 | 瞋 | 榴 | 朗 | 拜 | 寸 | 柏 | 伐 | 舛 | 秩 | 官 | 刀 | 青 | 代 | 語 | 叫 | 污 | 的 | 晶 | 碼 | 惆 | 衲 | 唻 | 昏 |
| 朝 | 什 | 君 | 開 | 軸 | 叩 | 昌 | 胡 | 府 | 力 | 九 | 惆 | 帝 | 馬 | 百 | 的 | 格 | 奸 | 佣 | 咱 | 司 | 上 | 安 | 謫 | 岳 |
| 朝 | 什 | 君 | 開 | 軸 | 叩 | 昌 | 胡 | 府 | 力 | 九 | 惆 | 帝 | 馬 | 百 | 的 | 格 | 奸 | 佣 | 咱 | 司 | 上 | 安 | 謫 | 岳 |
| 朝 | 什 | 君 | 開 | 軸 | 叩 | 昌 | 胡 | 府 | 力 | 九 | 惆 | 帝 | 馬 | 百 | 的 | 格 | 奸 | 佣 | 咱 | 司 | 上 | 安 | 謫 | 岳 |
| 甲 | 頭 | 坊 | 中 | 呷 | 祖 | 呼 | 調 | 月 | 惆 | 訐 | 圖 | 計 | 方 | 听 | 福 | 呻 | 訇 | 埔 | 順 | 酣 | 行 | 哺 | 干 | 王 |
| 甲 | 頭 | 坊 | 中 | 呷 | 祖 | 呼 | 調 | 月 | 惆 | 訐 | 圖 | 計 | 方 | 听 | 福 | 呻 | 訇 | 埔 | 順 | 酣 | 行 | 哺 | 干 | 王 |
| 靖 | 呀 | 肋 | 謳 | 艙 | 侄 | 屠 | 日 | 閃 | 但 | 署 | 們 | 昔 | 兵 | 門 | 蹦 | 闊 | 加 | 囧 | 諳 | 凹 | 彪 | 恫 | 伯 | 呎 |
| 靖 | 呀 | 肋 | 謳 | 艙 | 侄 | 屠 | 日 | 閃 | 但 | 署 | 們 | 昔 | 兵 | 門 | 蹦 | 闊 | 加 | 囧 | 諳 | 凹 | 彪 | 恫 | 伯 | 呎 |
| 青 | 彰 | 陳 | 用 | 刊 | 砒 | 哮 | 中 | 漂 | 愣 | 耗 | 捕 | 駒 | 助 | 鞫 | 玼 | 叫 | 喉 | 貝 | 串 | 吋 | 林 | 柳 | 痹 | 昌 |
| 青 | 彰 | 陳 | 用 | 刊 | 砒 | 哮 | 中 | 漂 | 愣 | 耗 | 捕 | 駒 | 助 | 鞫 | 玼 | 叫 | 喉 | 貝 | 串 | 吋 | 林 | 柳 | 痹 | 昌 |
| 割 | 佔 | 惓 | 閭 | 睚 | 短 | 曰 | 另 | 朋 | 輻 | 筵 | 瞄 | 刊 | 倍 | 甜 | 邛 | 叨 | 討 | 閨 | 賜 | 袖 | 猖 | 託 | 侷 | 于 |
| 割 | 佔 | 惓 | 閭 | 睚 | 短 | 曰 | 另 | 朋 | 輻 | 筵 | 瞄 | 刊 | 倍 | 甜 | 邛 | 叨 | 討 | 閨 | 賜 | 袖 | 猖 | 託 | 侷 | 于 |
| 附 | 時 | 蚪 | 誇 | 勃 | 謝 | 漚 | 刪 | 咕 | 湘 | 門 | 悄 | 粃 | 晶 | 閣 | 豆 | 刀 | 軻 | 若 | 闕 | 聒 | 柯 | 苒 | 籍 | 漕 |
| 附 | 時 | 蚪 | 誇 | 勃 | 謝 | 漚 | 刪 | 咕 | 湘 | 門 | 悄 | 粃 | 晶 | 閣 | 豆 | 刀 | 軻 | 若 | 闕 | 聒 | 柯 | 苒 | 籍 | 漕 |

Figure 1: Visual comparison of the results of the first to fifth styles. The first row shows the source characters. The second row shows the characters generated by ZiGAN. And the third row shows the ground truth.

|   |   |   |   |   |   |   |   |   |   |   |   |   |   |   |   |   |   |   |   |   |   |   |   |   |
|---|---|---|---|---|---|---|---|---|---|---|---|---|---|---|---|---|---|---|---|---|---|---|---|---|
| 詳 | 晰 | 兵 | 瞄 | 單 | 尉 | 捕 | 垢 | 滴 | 胸 | 映 | 恒 | 卦 | 迫 | 踹 | 忤 | 螞 | 半 | 胭 | 回 | 兵 | 川 | 門 | 鯛 | 誼 |
| 詳 | 晰 | 兵 | 瞄 | 單 | 尉 | 捕 | 垢 | 滴 | 胸 | 映 | 恒 | 卦 | 迫 | 踹 | 忤 | 螞 | 半 | 胭 | 回 | 兵 | 川 | 門 | 鯛 | 誼 |
| 誼 | 晰 | 昌 | 腓 | 邗 | 伴 | 趁 | 守 | 守 | 叵 | 附 | 謂 | 計 | 悖 | 穎 | 巾 | 長 | 佞 | 森 | 劭 | 聘 | 律 | 肝 | 下 | 軍 |
| 誼 | 晰 | 昌 | 腓 | 邗 | 伴 | 趁 | 守 | 守 | 叵 | 附 | 謂 | 計 | 悖 | 穎 | 巾 | 長 | 佞 | 森 | 劭 | 聘 | 律 | 肝 | 下 | 軍 |
| 杭 | 彈 | 佰 | 貝 | 順 | 棚 | 拆 | 別 | 輯 | 確 | 麒 | 榜 | 彰 | 燭 | 邑 | 侵 | 風 | 方 | 閃 | 敖 | 喃 | 閉 | 暑 | 埃 | 侶 |
| 杭 | 彈 | 佰 | 貝 | 順 | 棚 | 拆 | 別 | 輯 | 確 | 麒 | 榜 | 彰 | 燭 | 邑 | 侵 | 風 | 方 | 閃 | 敖 | 喃 | 閉 | 暑 | 埃 | 侶 |
| 暗 | 勒 | 刑 | 詞 | 閏 | 叩 | 捌 | 碘 | 例 | 謳 | 甫 | 勛 | 鴿 | 肝 | 倘 | 月 | 恂 | 胛 | 軌 | 輻 | 肱 | 精 | 儲 | 街 | 街 |
| 暗 | 勒 | 刑 | 詞 | 閏 | 叩 | 捌 | 碘 | 例 | 謳 | 甫 | 勛 | 鴿 | 肝 | 倘 | 月 | 恂 | 胛 | 軌 | 輻 | 肱 | 精 | 儲 | 街 | 街 |
| 刀 | 噬 | 伸 | 梗 | 樽 | 冰 | 姬 | 昨 | 做 | 煥 | 微 | 敫 | 汲 | 巧 | 沸 | 咧 | 理 | 僵 | 咄 | 擻 | 板 | 喘 | 尉 | 獮 | 囁 |
| 刀 | 噬 | 伸 | 梗 | 樽 | 冰 | 姬 | 昨 | 做 | 煥 | 微 | 敫 | 汲 | 巧 | 沸 | 咧 | 理 | 僵 | 咄 | 擻 | 板 | 喘 | 尉 | 獮 | 囁 |
| 狎 | 棒 | 哏 | 泐 | 泐 | 哺 | 汜 | 把 | 弛 | 樞 | 荆 | 托 | 翊 | 晁 | 琅 | 奔 | 丞 | 侗 | 懔 | 帥 | 樞 | 嘲 | 恹 | 慚 | 咻 |
| 狎 | 棒 | 哏 | 泐 | 泐 | 哺 | 汜 | 把 | 弛 | 樞 | 荆 | 托 | 翊 | 晁 | 琅 | 奔 | 丞 | 侗 | 懔 | 帥 | 樞 | 嘲 | 恹 | 慚 | 咻 |
| 吠 | 唱 | 叭 | 飲 | 噪 | 恢 | 昨 | 毡 | 廂 | 礪 | 剔 | 欺 | 欺 | 欺 | 嚇 | 吓 | 吓 | 慢 | 啡 | 呐 | 你 | 喧 | 舜 | 勤 | 嗽 |
| 吠 | 唱 | 叭 | 飲 | 噪 | 恢 | 昨 | 毡 | 廂 | 礪 | 剔 | 欺 | 欺 | 欺 | 嚇 | 吓 | 吓 | 慢 | 啡 | 呐 | 你 | 喧 | 舜 | 勤 | 嗽 |
| 涸 | 肋 | 捱 | 辦 | 焗 | 咧 | 稿 | 歉 | 炬 | 吹 | 佐 | 次 | 笑 | 映 | 叮 | 腰 | 輯 | 砂 | 鴿 | 畦 | 昔 | 呖 | 獅 | 豚 | 碾 |
| 涸 | 肋 | 捱 | 辦 | 焗 | 咧 | 稿 | 歉 | 炬 | 吹 | 佐 | 次 | 笑 | 映 | 叮 | 腰 | 輯 | 砂 | 鴿 | 畦 | 昔 | 呖 | 獅 | 豚 | 碾 |

Figure 2: Visual comparison of the results of the sixth to ninth styles. The first row shows the source characters. The second row shows the characters generated by ZiGAN. And the third row shows the ground truth.
